# Supplementary material for: Limitations of Piecewise Linearity for Efficient Robustness Certification
Source: arXiv:2301.08842 source file (2023-01-21)
Supplement: Supplementary file 1 [file supplementary_sphere_approx.tex]

% !TEX root=./main.tex

\section{Rounding Corners by Approximating Hyper-spheres}
\label{sec:sphere_approx}

% ... analyzing the decision boundary of a real-world example would be prohibitively expensive. Furthermore, the inability to solve the ``corner problem'' with reasonable capacity may lead the network to make other compromises that avoid corners but lead to sub-optimality in a way that is fundamentally caused by the same principle.

We consider the following thought experiment to provide some slightly more specific intuition regarding the additional capacity required to tightly certify regions near sharp ``corners'' in a piecewise-linear model's decision boundary.
As in Section~\ref{sec:corners}, we ...
The points for which certification is loose falls within the hypercube of width $\epsilon$, just opposite the corner.
The true robust frontier in this region is given by the intersecting orthant of the hypersphere of radius $\epsilon$...
In order to ... we must approximate this spherical orthant using linear hyperplanes that do not interse
